# Supplementary material for: Color Matching Using Hypernetwork-Based Kolmogorov-Arnold Networks
Source: arXiv:2503.11781 source file (2025-03-14)
Supplement: Supplementary file 1 [file 1_splines_an.tex]

\section{KANs and Color-Matching Problem}
\label{sec:splines}

%In this section, we detail the mathematical reasoning behind why a single KAN layer is sufficient for our color-matching task.

An abstract camera Image Signal Processing (ISP) pipeline can be represented as a combination of linear and non-linear transformations~\cite{AN1, AN3, AN9, AN4, finlayson2017color}. Specifically, the image formation process can be represented mathematically as:  
\begin{equation}\label{eq:isp}
{I}_{\text{rgb}} = T({I}_{\text{raw}} \mathbf{C}),
\end{equation}  
\noindent
where ${I}_{\text{raw}}$ is the input image in the camera raw space, ${I}_{\text{rgb}}$ is the output image in one of the display standard spaces (\textit{e.g.}, sRGB), $\mathbf{C}$ represents the linear component of the ISP pipeline, and ${T}$ implements the non-linear transformations, such as tone mapping, gamut mapping, image enhancement \textit{etc}
~\cite{zhang2023lookup}.  

Now, consider performing color matching between two images of the same scene, processed through different ISP pipelines, denoted as $ISP_x$ and $ISP_y$. Based on Eq.~\ref{eq:isp}, the color matching of two pixels $x$ and $y$ in the corresponding images, $X = ISP_x(I_\text{raw})$ and $Y = ISP_y(I_\text{raw})$,  can be represented as:  
\begin{equation}\label{eq:translation}
y = T_{y}(T_{x}^{-1}(x) \mathbf{L}),
\end{equation}  
\noindent
where $\mathbf{L}$ represents a linear transformation, and ${T}_{x}$ and ${T}_{y}$ are the non-linear color transformations of the respective ISPs.

According to the Color Homography Theorem~\cite{finlayson2017color}, the non-linear transformations $T_{x}$ and $T_{y}$ in Eq.~(\ref{eq:translation}) can be represented by a shading matrix, enabling their replacement with a single operation:  
\begin{equation}\label{eq:translation_final}
y = T(x) \mathbf{L}.
\end{equation}  

To achieve an accurate approximation of $T(x)$, choosing a plausible parametric space for a model is essential. A straightforward approach is to implement gamma correction, as suggested in~\cite{AN2}. However, gamma correction alone is insufficient to address the non-linearity of ISP~\cite{afifi2019color}, and in ~\cite{AN1} polynomial approximation is proposed. 

\begin{equation}
\hat{y}_j = \sum_{i=0}^{2} \left( l_{ji} \sum_{m=0}^{n-1} p_{ijm} (x_i)^m\right),
\label{eq:splines_for_color}
\end{equation}

More general approach of B-spline-based approximation of (\ref{eq:translation_final})  could be represented for color channels $i$ and $j$ of source and target images as:
\begin{equation}
\hat{y}_j = \sum_{i=0}^{2} \left( l_{ji} \sum_{m=0}^{G+k-1} c_{ijm} B_{ijm}(x_i)\right),
\label{eq:splines_for_color}
\end{equation}
where $l_{ji}$ are elements of matrix $\mathbf{L}$, $c_{ijm}$ are spline coefficients and $B_{ijm}(x_i)$ are b-spline basis functions of order $k$ and grid size $G$.
This spline approximation could be directly implemented using KANs to approximate the non-linear component $T(\cdot)$, as it offers several advantages.  

Firstly, KAN approximates (\ref{eq:translation_final}) as physically informed neural network which allows SGD-based training process and could be integrated into end-to-end deep learning pipeline, while traditional polynomial approximations of ~\cite{AN1} and~\cite{AN2} relies on standalone global optimizers.  
KAN is comparable to MLP; however, instead of learnable weights, it has learnable activation functions on edges, and the summation of the resultant learned function's output is performed at the nodes.  
Unlike MLPs, which rely on the Universal Approximation Theorem, KANs, accordingly to theorem 2.1 of~\cite{AN6}, provide smooth spline approximation which is important for accurate and artifacts-free color matching process [I''l try to find any ref].
%\cite{kolmogorov:superposition}.

The original KAN implementation~\cite{AN6} used a residual connection mechanism and expressed
%the activation function \(\phi(x)\) 
as the combination of the basis function \(silu(x)\) and the B-spline function. The final equation for a KAN layer  with $n_{\text{in}}$ inputs and $n_{\text{out}}$ outputs can be represented as:

{\scriptsize
\begin{equation}
\hat{y}_j = \sum_{i=0}^{n_{\text{in}}-1} \left(u_{ij} silu(x_i) + v_{ij} \sum_{m=0}^{G+k-1} c_{ijm} B_{ijm}(x_i)\right)
\label{eq:kan_layer}
\end{equation}
}

\noindent where, ${x_i}$, ${\hat{y}_j}$ represents the input and output components, respectively, ${silu(.)}$ is residual activation function, $B_{ijm}(.)$ are the b-spline basis functions, and $u_{ij}$, $v_{ij}$, $c_{ijm}$ are KAN layer parameters, and $j = 0,1, \cdots, n_{\text{out}}-1$, $G$ and $k$ denotes the grid size and spline order, respectively. In our method, the KAN layer no longer has its own trainable parameters ($u_{ij}$, $v_{ij}$, $c_{ijm}$). Instead, these parameters are dynamically provided by the hypernetwork (i.e., the generator network) for each pixel of the image. The representation (\ref{eq:splines_for_color})  corresponds to (\ref{eq:kan_layer})  with $u_{ij} = 0$ which justify our implementation of (\ref{eq:translation_final}) by Kolmogorov-Arnold Networks.

For our implementation, we use a single KAN layer configured with an input size of $n_{\text{in}}=3$, output size of $n_{\text{out}}=3$, spline order $k = 3$, and a grid size of $G = 5$. It can be represented as:
\begin{equation}
\hat{y}_j = \sum_{i=0}^{2} \left(u_{ij} silu(x_i) + v_{ij} \sum_{m=0}^{7} c_{ijm} B_{ijm}(x_i)\right).
\end{equation}
