# Supplementary material for: Color Matching Using Hypernetwork-Based Kolmogorov-Arnold Networks
Source: arXiv:2503.11781 source file (2025-03-14)
Supplement: Supplementary file 2 [file 6_Additional_Ablation.tex]

\section{Ablation study}
\label{sec:ablation}

\begin{table}[t]
\centering
\caption{\textbf{Ablation results of the impact of the compression operation on vectors of attention} on our dataset.}
\label{supp-tab:study_kqv}
\begin{tabular}{c|cc|cc}
\toprule
Modification & PSNR& SSIM & $\Delta E$& SSIM$\uparrow$   \\
\midrule
w/o compression & 00.00  & 0.00 & 0.00 \\
w. compression & 00.00  & 0.00 & 0.00  \\

\bottomrule
\end{tabular}
\end{table}
